# Supplementary material for: Tail-GAN: Learning to Simulate Tail Risk Scenarios
Source: arXiv:2203.01664 source file (2025-05-16)
Supplement: Supplementary file 1 [file appendix.tex]

\section{Additional results from Section \ref{sec:model_validation}}

\begin{figure}[H]
\centering
\subfigure[Performance evaluated with static portfolios.]{ \label{fig:synthetic_is_static}
\includegraphics[width=.48\textwidth]{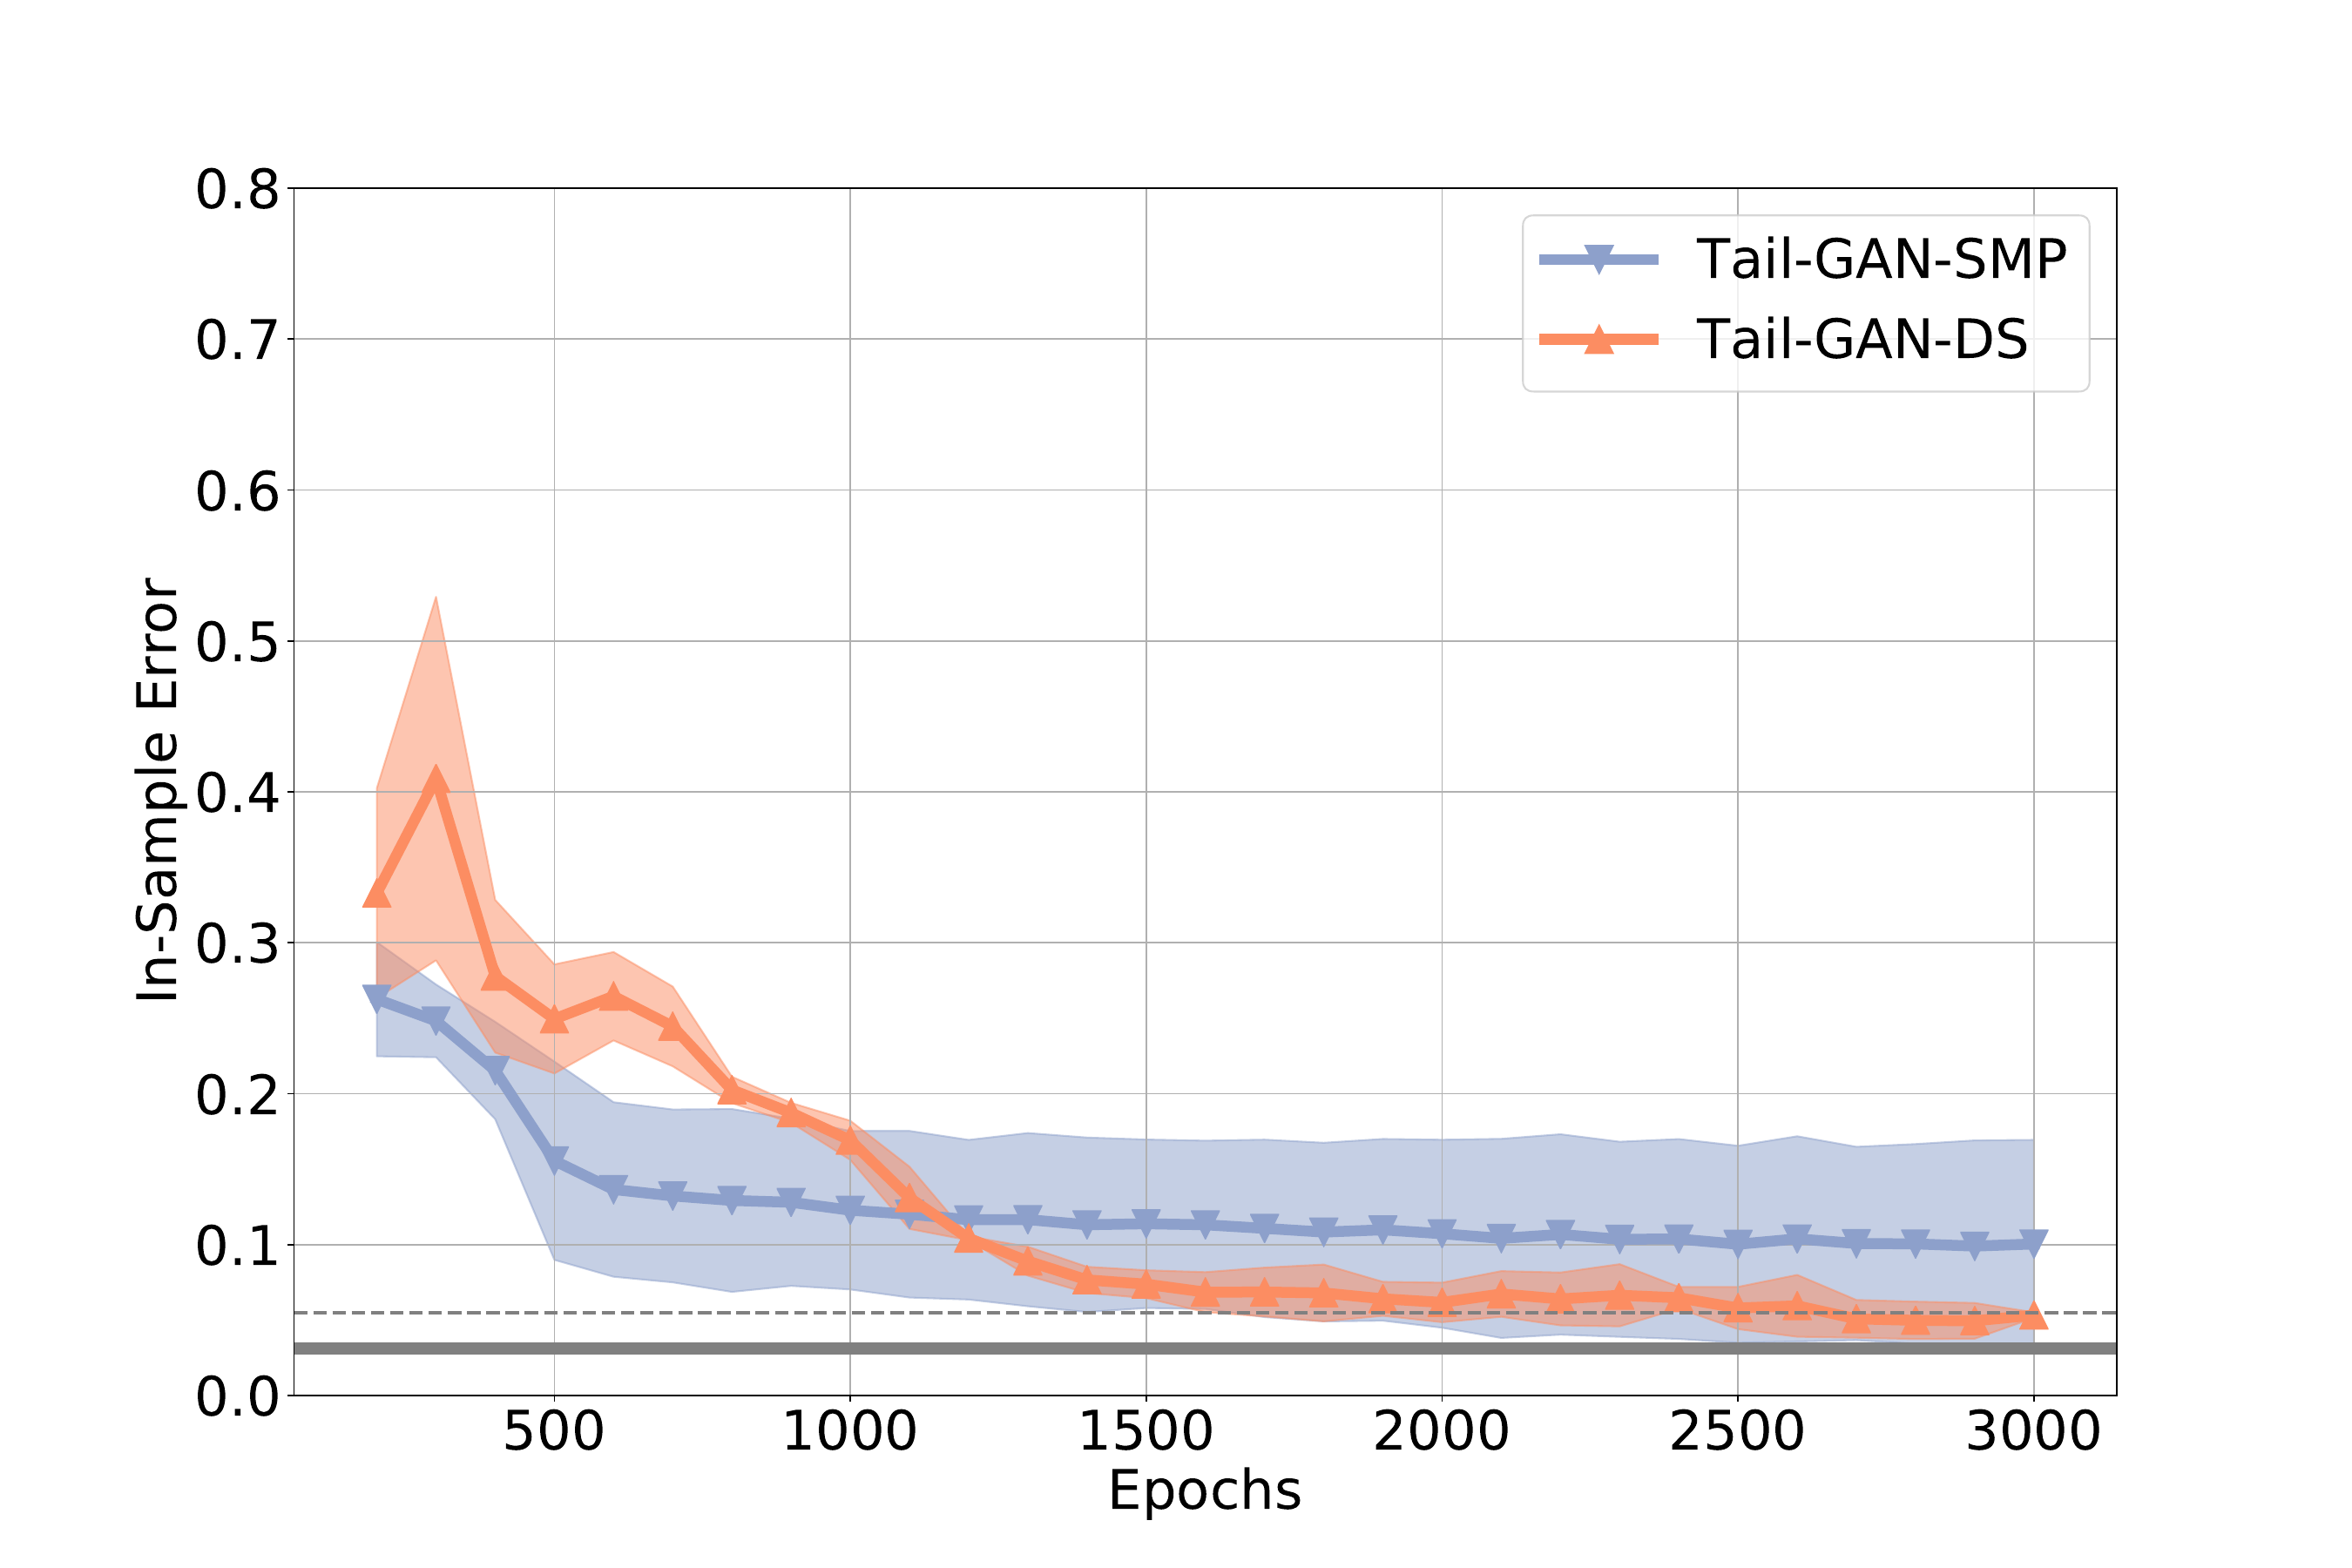}
}
\subfigure[Performance evaluated with all strategies.]{ \label{fig:synthetic_is_all}
\includegraphics[width=.48\textwidth]{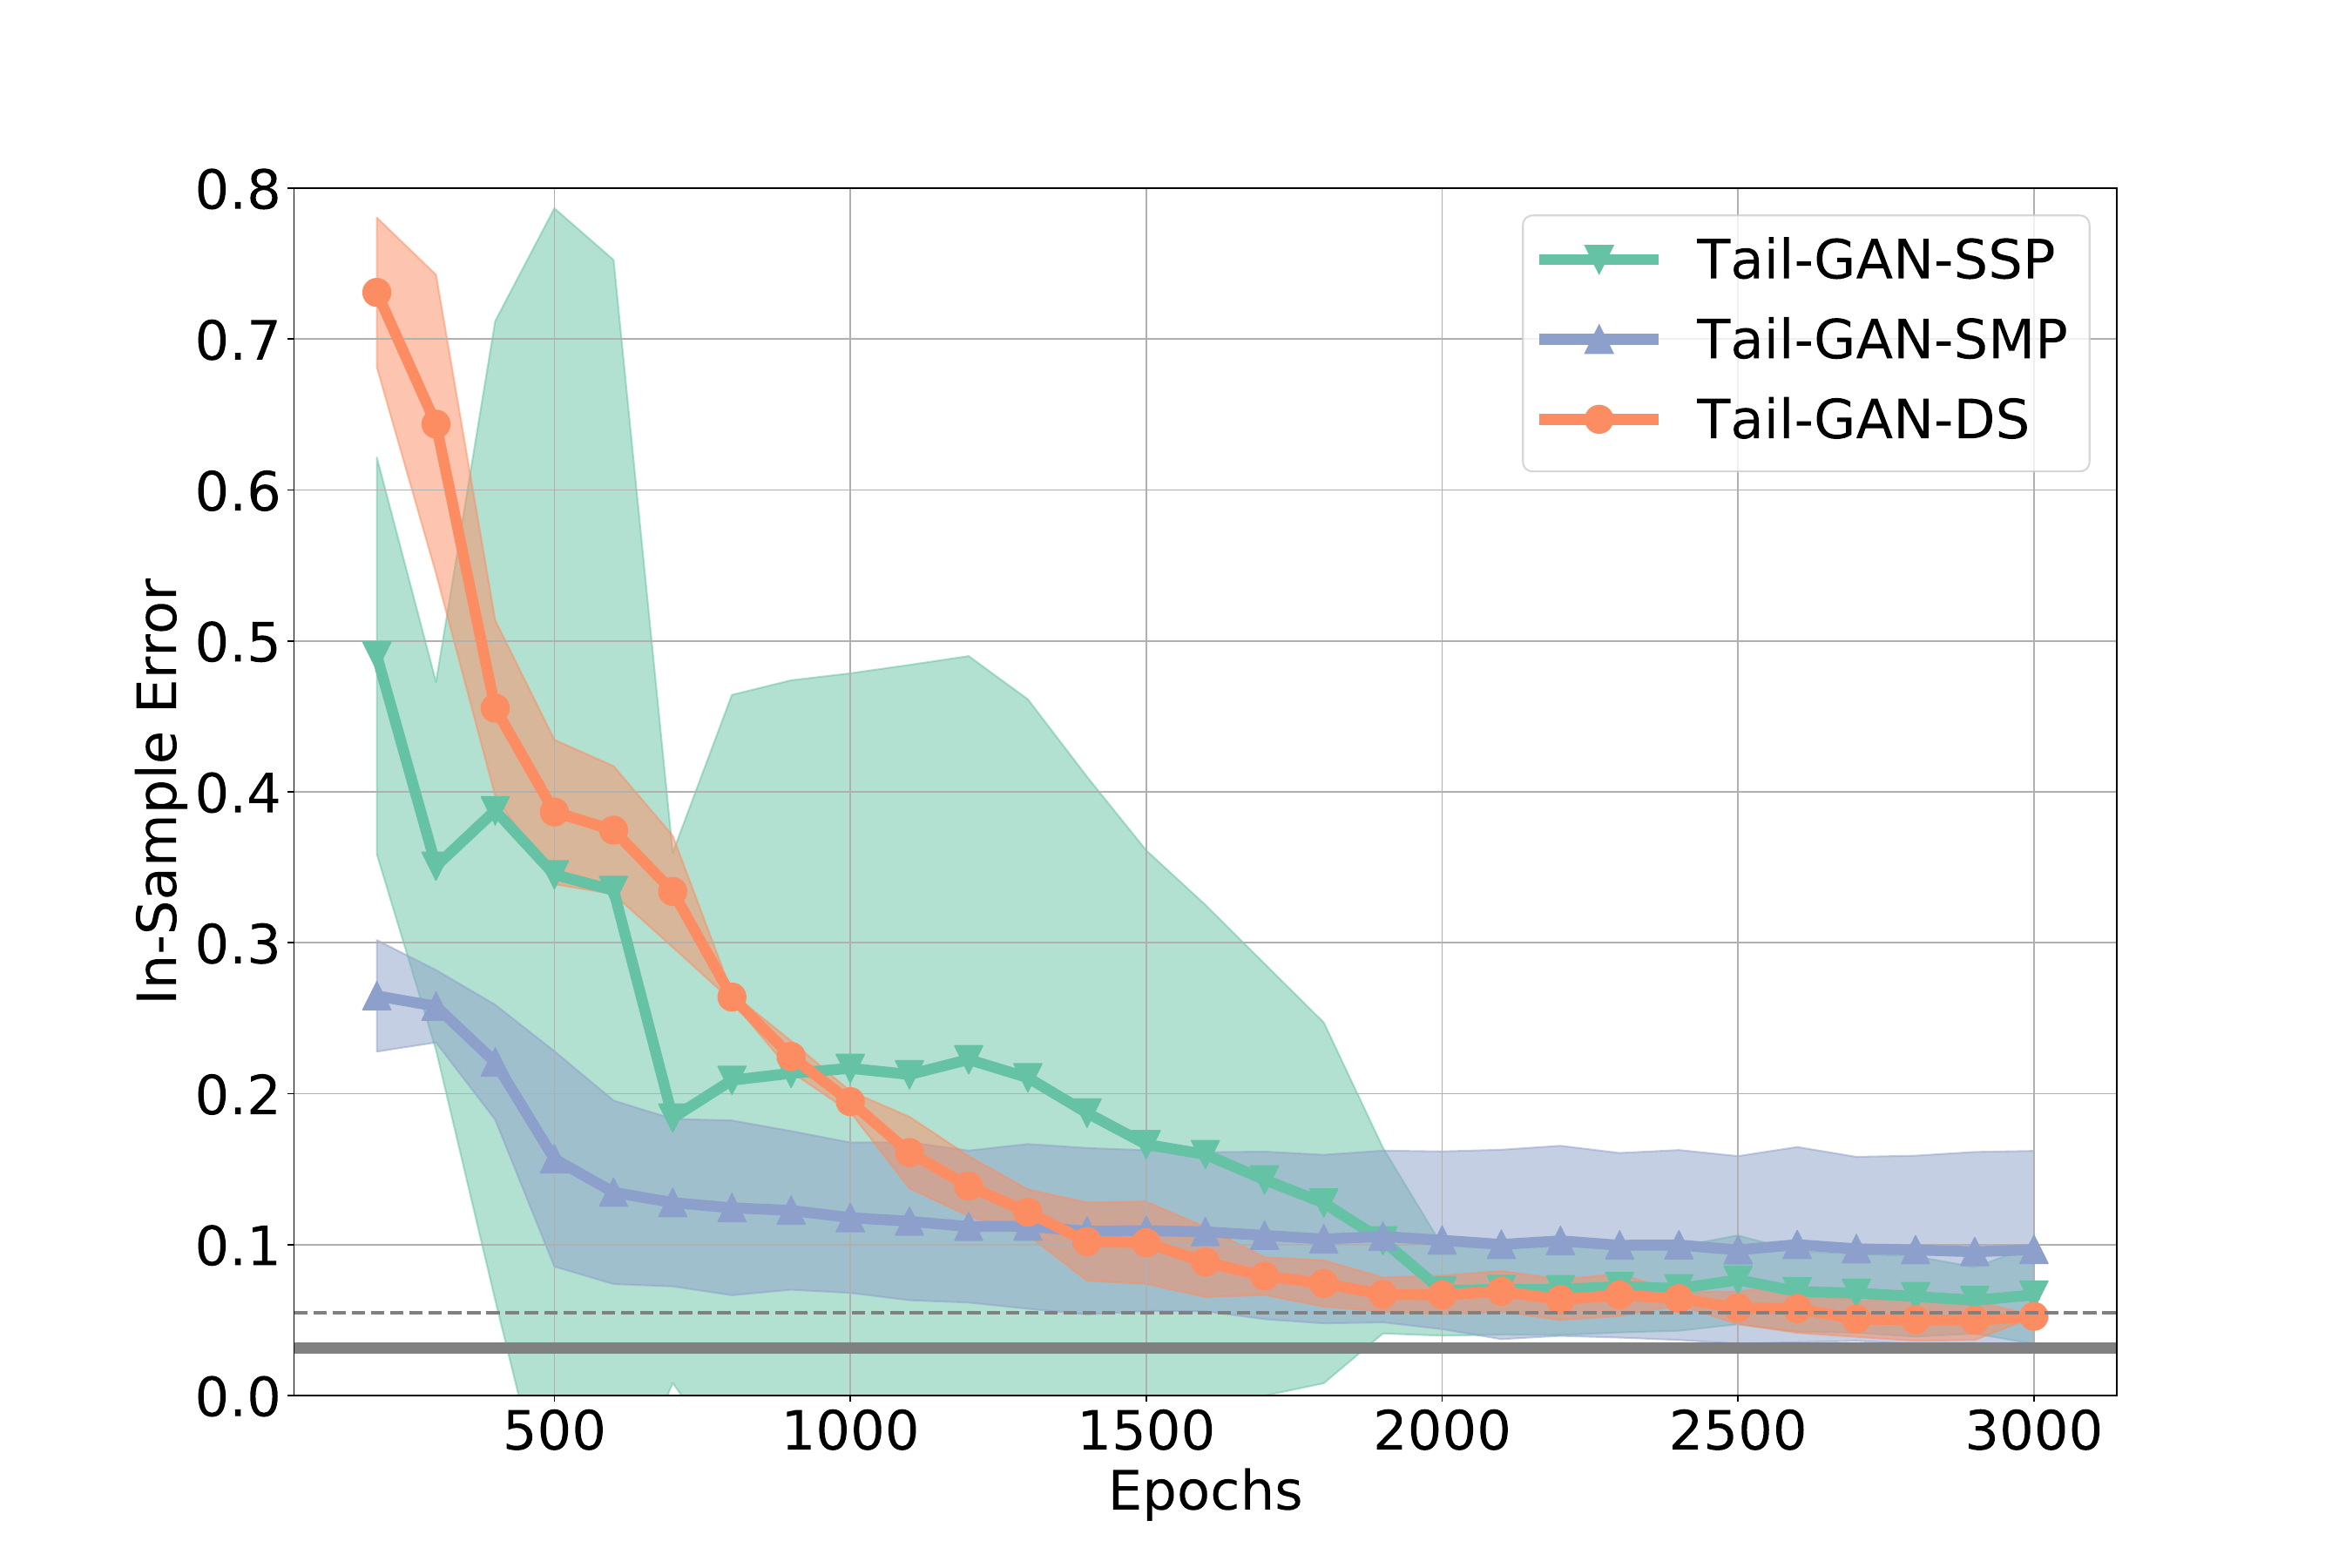}
}
\caption{In-sample performance ${\rm RE}(1000)$. Grey horizontal line: average simulation error {${\rm SE}(1000)$}. Dotted line: average simulation error plus one standard deviation. Each experiment is repeated 5 times with different random seeds. The performance is visualized with mean (solid lines) and standard deviation (shaded areas).} \label{fig:model_validation_performance}
\end{figure}

\paragraph{Scalability.}
Given the fact that relative error is unstable when evaluating low volatility portfolios\RX{not very clear to me}, we also compare the absolute error 
\begin{equation}
    {\rm AE}(n) = \frac{1}{2K} \sum_{k=1}^{K} \left( |{\rm VaR}_{\alpha}\left( \Pi^k\#\,\mathbb{P}_{G}^{(n)}\right) - {\rm VaR}_{\alpha}\left(\Pi^k\#\, \mathbb{P}_{r}\right)| + |{\rm ES}_{\alpha}\left( \Pi^k\#\,\mathbb{P}_{G}^{(n)}\right) - {\rm ES}_{\alpha}\left(\Pi^k\#\, \mathbb{P}_{r}\right)|\right).
\end{equation}

\begin{figure}[H]
\centering
\includegraphics[width=.65\textwidth]{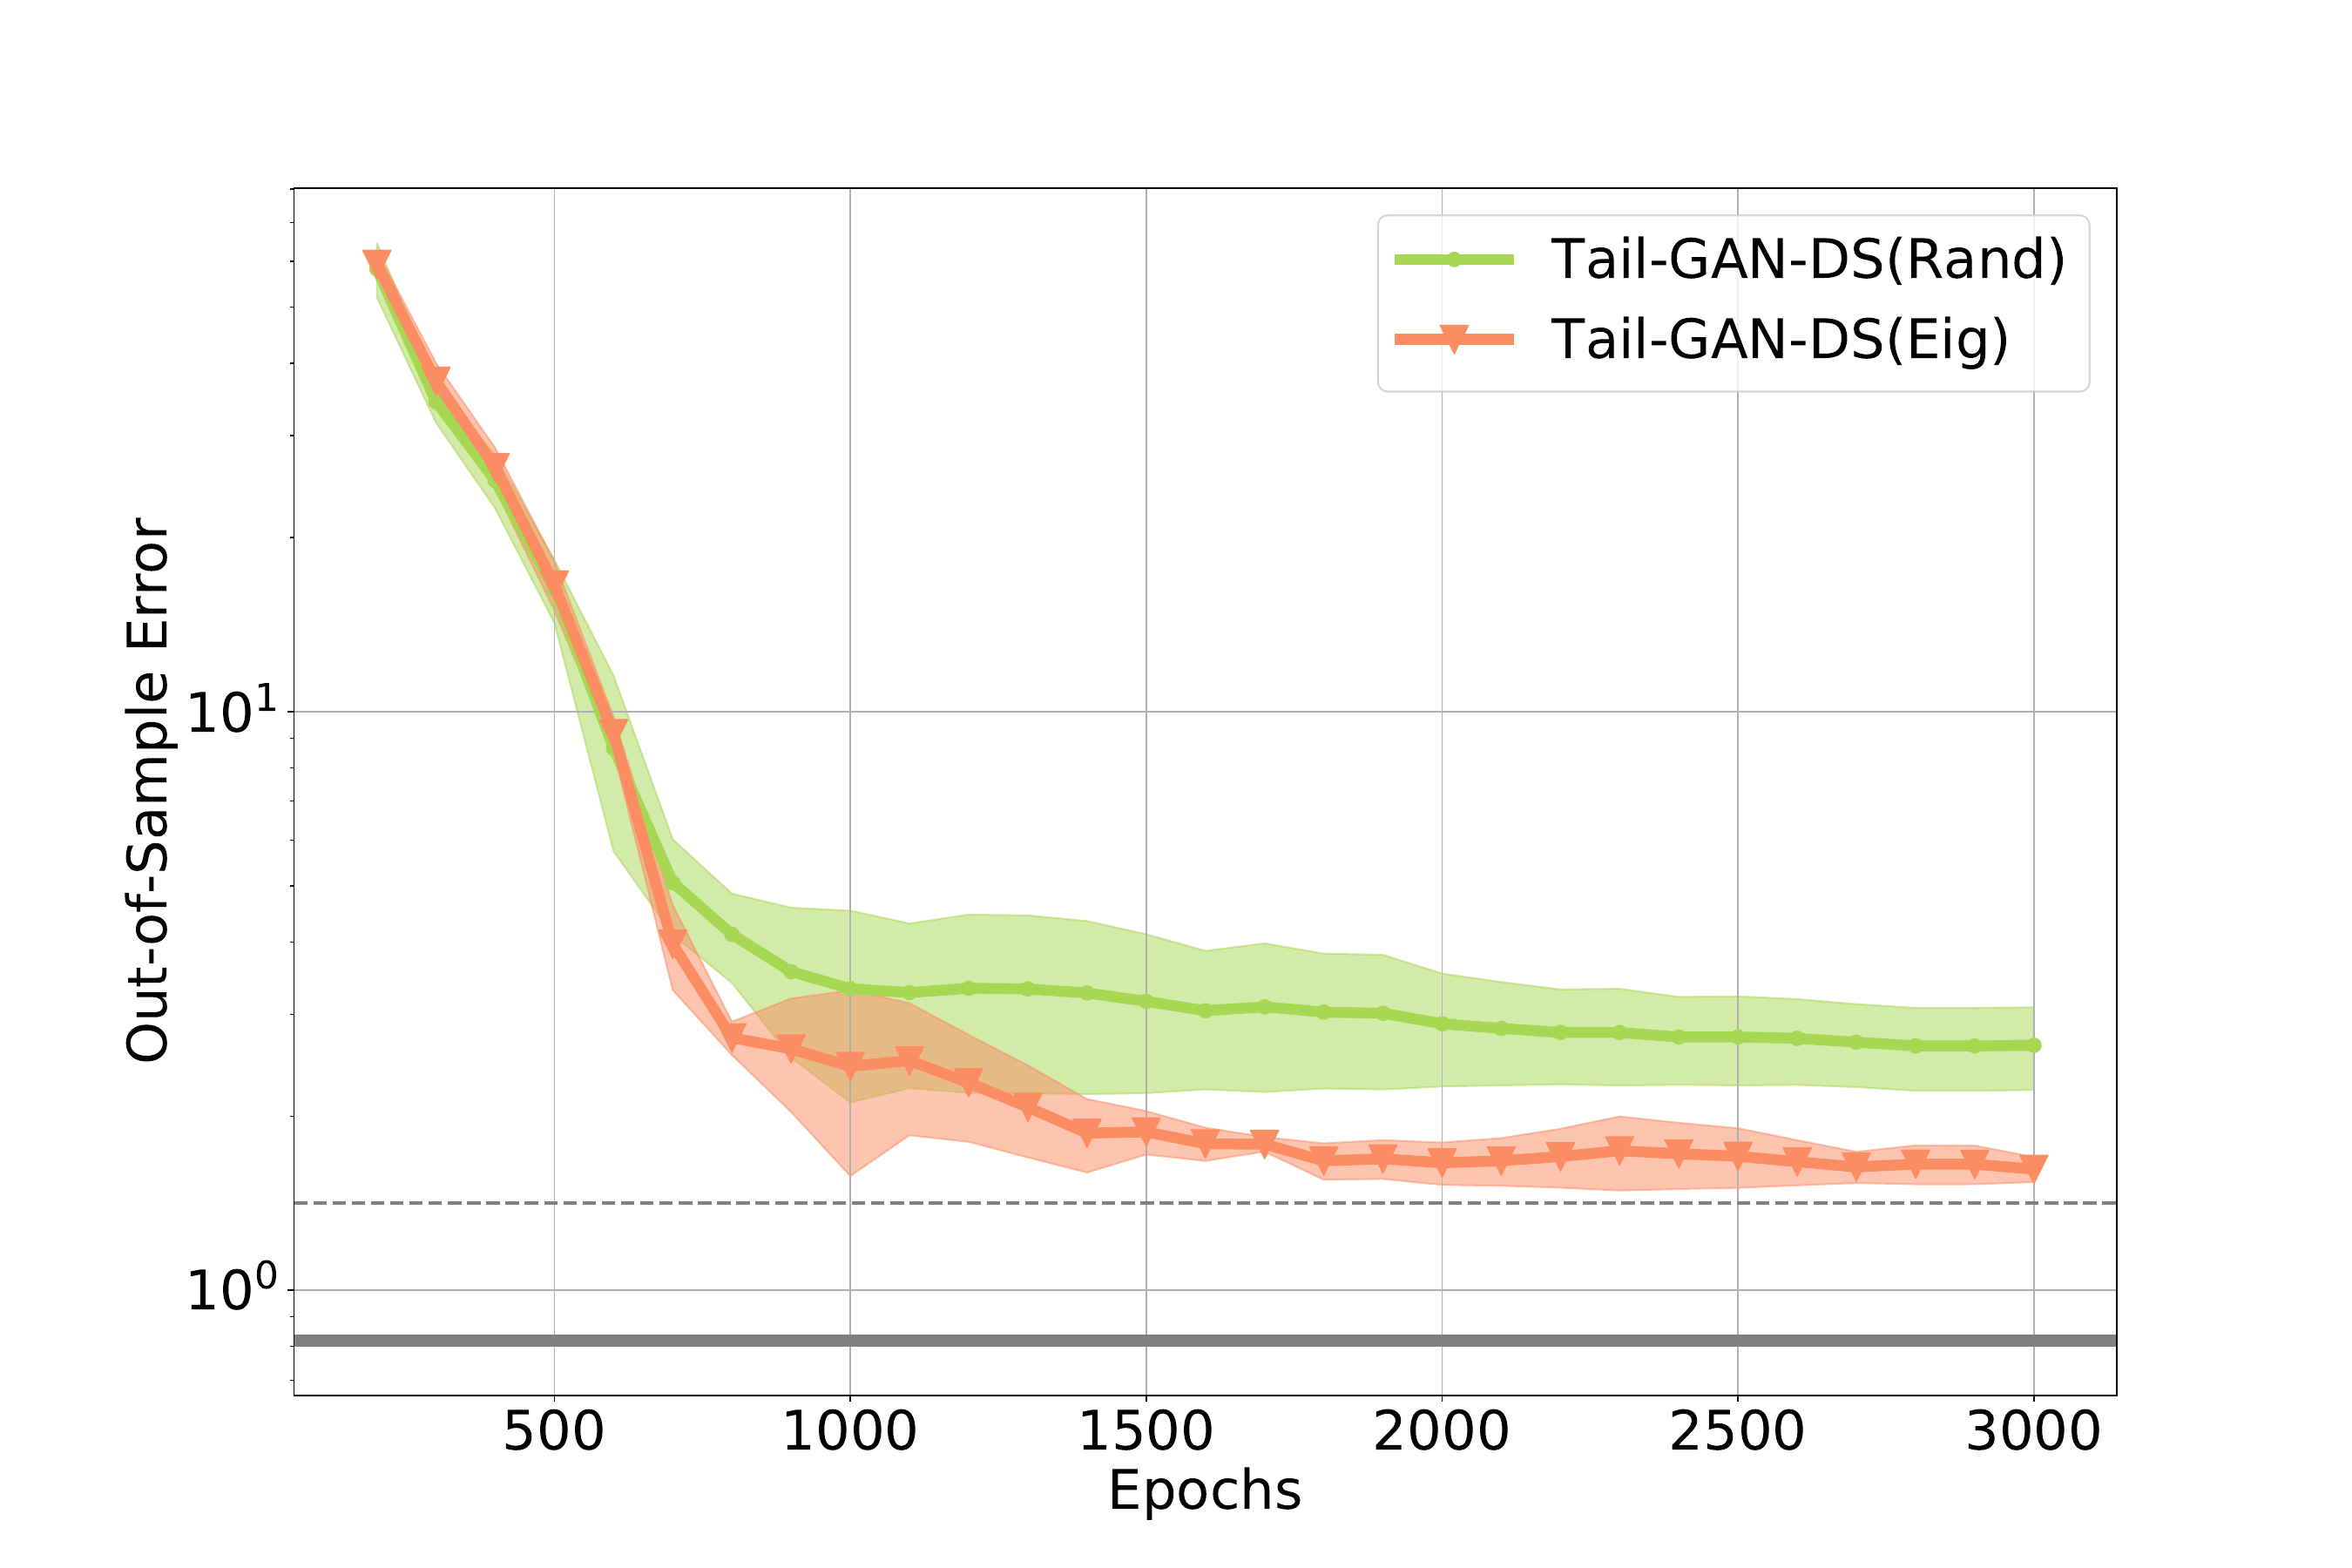}
\caption{Out-of-sample Absolute Error evaluated with all strategies. Grey horizontal line: average simulation error. Dotted line: average simulation error plus one standard deviation. Each experiment is repeated 5 times with different random seeds. The performance is visualized with mean (solid lines) and standard deviation (shaded areas).}
\label{fig:syn_eig_ae}
\end{figure}

\section{Derivatives with respect to the loss function} \label{sec:derivatives}
Recall the loss of the discriminator and the generator used in Algorithm \ref{alg:algorithm1}, i.e. $\mathcal{L}_D(\delta)$ and $\mathcal{L}_G(\gamma)$. According to the chain rule, we have 
\begin{eqnarray}
\frac{\partial \mathcal{L}_D(\delta)}{\partial {\delta}} &=& \frac{1}{K\,N_B}\sum_{k=1}^K \sum_{n \in \mathcal{B}_j} \left[
\left. \left( \frac{\partial S_{\alpha}}{\partial v_k}\frac{\partial v_k}{\partial {\delta}}+ \frac{\partial S_{\alpha}}{\partial e_k} \frac{\partial e_k}{\partial {\delta}} \right) \right|_{\substack{({v}_{k}, {e}_{k})=D_{{\delta}}(\Pi^k(G_{{\gamma}}({\pmb{z}_{i}})),i\in[N_B])\\
x = \Pi^{k}(\pmb{p}_{n})}} \nonumber \right. \\
&&-  
\left. \left. \left( \frac{\partial S_{\alpha}}{\partial v_k}\frac{\partial v_k}{\partial {\delta}}+ \frac{\partial S_{\alpha}}{\partial e_k} \frac{\partial e_k}{\partial {\delta}} \right) \right|_{\substack{({v}_{k}, {e}_{k})=D_{{\delta}}(\Pi^k(\pmb{p}_i), i \in \mathcal{B}_j)  \\
x = \Pi^{k}(\pmb{p}_{n})}} \nonumber \right], \\
\frac{\partial \mathcal{L}_G(\gamma)}{\partial {\gamma}} &=& \frac{1}{K\,N_B}\sum_{k=1}^K \sum_{n \in \mathcal{B}_j} \left[ \left. \left(\frac{\partial S_{\alpha}}{\partial v_k} \frac{\partial v_k}{\partial {\pmb{q}_i}} \frac{\partial {\pmb{q}_i}}{\partial {\gamma}} + \frac{\partial S_{\alpha}}{\partial e_k} \frac{\partial e_k}{\partial {\pmb{q}_i}} \frac{\partial {\pmb{q}_i}}{\partial {\gamma}} \right)\right|_{\substack{
({v}_{k}, {e}_{k})=D_{{\delta}}( \Pi^{k}({\pmb{q}_i}), i \in [N_B]) \\
{\pmb{q}_i} = G_{\gamma}(\tilde{\pmb{z}}_i) \\
x = \Pi^{k}(\pmb{p}_{n})}} \right]. \nonumber
\end{eqnarray}

\section{Summary of Notations}
\begin{table}[H]
    \centering
    \resizebox{0.75\textwidth}{!}{\begin{tabular}{ll}  
\hline
Symbol & Description \\\hline
$X \sim \mu$ & Random variable with distribution $\mu$\\
$\alpha$ & A specific quantile \\
$\mbox{VaR}_{\alpha}(\mu)$ & Value at Risk of distribution $\mu$ at $\alpha$ level \\
$\mbox{ES}_{\alpha}(\mu)$ & Expected Shortfall of distribution $\mu$ at $\alpha$ level \\
$S_{\alpha}(v,e,x)$ & Score \\
$H_1, H_2$ & Component functions in Score function \\
$M$ & Number of assets \\
$T$ & Periods \\
$\Delta$ & Duration of intervals \\
{{$\pmb{p} = \{(p_{m,t})_{t=1}^{T}\}_{m=1}^M$}} & Random matrix of price \\
$\pmb{p}_1, \cdots, \pmb{p}_N$ & $N$ IID samples of $\pmb{p}$ \\
$\mathbb{P}_r$ & Theoretical distribution of $\pmb{p}$ \\
$\mathbb{P}_r^{(n)}$ & Empirical distribution of $\mathbb{P}_r$ with $n$ samples\\
% $\hat{\mathbb{P}}^{N}_r$ & Empirical distribution of $\pmb{p}$ \\
$N_z$ & Dimension of noise \\
$L$ & Number of layers \\
$n_l$ & Width of the $l$-th layer \\
{{$\pmb{z}$}} & Input of the generator \\
$\pmb{W} = (\pmb{W}_l)_{l=1}^{L}, \pmb{b}=(\pmb{b}_l)_{l=1}^{L}$ & Parameters in the NN \\
$\sigma(\cdot)$ & Activation function \\
$G$ & Generator \\
$\mathcal{G}_{NN}$ & Class of generators \\
$\gamma$ & Parameters of Generator $G_{\gamma}(\cdot)$ (or $G(\cdot; \gamma)$)\\ %\hline
$\mathbb{P}_{G}$ & Theoretical distribution of price series generated by $G$ \\
$\mathbb{P}_{G}^{(n)}$ & Empirical distribution of $\mathbb{P}_{G}$ with $n$ samples\\
$K$ & Number of trading strategies \\
$\pmb{w} = (w_i)_{i=1}^{M}$ & Shares of $M$ assets in a static portfolio or dynamic strategy \\
$p_t(\pmb{w})$ & Market price of a combination $\pmb{w}$ \\
$A_t$ & Moving average estimator \\
$s_t(\pmb{w})$ & Trading signals \\
$s_U, s_L$ & Threshold to buy or short \\
$\overline{p}_t(\pmb{w},d)$ & Moving average price of the portfolio \\
$d_1, d_2$ & Durations of moving average estimator\\
$c$ & Cash budget \\ 
$\Pi^k$ & Strategy $k$ \\
{{$x^k = \Pi^{k}(\pmb{p})$}}& Final PnL of $\Pi^k$ at terminal time $T$\\
$\Pi^k\#\,\mathbb{P}_{r}$ & Theoretical distribution of $\Pi^{k}(\pmb{p})$ \\
$\Pi^k\#\,\mathbb{P}_{r}^{(n)}$ & Empirical distribution of $\Pi^k\#\,\mathbb{P}_{r}$ with $n$ samples \\
% $\mathbb{P}^{k}_{\text{PnL}, r}$ & Theoretical distribution of $\Pi^{k}(\pmb{p})$ \\
$\Pi^k\#\,\mathbb{P}_{G}$ & Theoretical distribution of $\Pi^{k}(G(\pmb{z}; \gamma))$  \\
$\Pi^k\#\,\mathbb{P}_{G}^{(n)}$ & Empirical distribution of $\Pi^k\#\,\mathbb{P}_{G}$ with $n$ samples \\
% $\mathbb{P}^{k}_{\text{PnL}, G} $ & Theoretical  distribution of $\Pi^{k}(G(\pmb{z}; \gamma))$ \\
$\pmb{\Pi} := (\Pi^1,\cdots,\Pi^K)$ & Mapping of all strategies \\%\hdashline
% $f_{\alpha}$ & Mapping $\alpha$-quantile VaR and ES values of distributions \\%\hline
$N_{B}$ & Number of PnL samples \\
{{$\{x^{k}_{i}\}_{i=1}^{N_{B}}$}} & PnL samples of strategy $k$\\
$\pmb{x}^{k} = (x^{k}_{i})_{i=1}^{N_{B}}$ & Vector of PnLs computed according to strategy $k$\\
$B(\pmb{x}^{k})$ & Absolute pairwise differences of the elements of $\pmb{x}^{k}$ \\
{{$\Gamma(\pmb{x}^{k})$}} & Permutation matrix of $\pmb{x}^{k}$ \\
$\mathcal{D}_{NN}$ & Class of discriminators \\
$\delta$ & Parameters of the discriminator $D_{\delta}(\cdot)$ (or $D(\cdot; \delta)$) \\\hline
\label{tab:notation}
\end{tabular}}
    \caption{Summary of Notations.} 
    \label{tab:notation}
\end{table}
